# Supplementary material for: Software-Hardware Co-Optimization for Computational Chemistry on Superconducting Quantum Processors
Source: arXiv:2105.07127 source file (2021-05-15)
Supplement: Supplementary file 1 [file appendix.tex]

\section{Quantitative Explanation of Section~\ref{sec:stringmatching}}\label{appendix:stringcompare}
In this appendix, we provide more clarification and intuition behind our heuristic parameter pruning approach on the UCCSD ansatz. We seek to eliminate those parameters that contribute the least to final measurement results. Doing this precisely for each parameter can be very complex.
Fortunately, in variational algorithms, we do not have to be very precise, as long as the optimization can converge in a reasonable amount of time. The key is to have enough parameters to explore the optimization space and move towards the answer by adjusting those parameters at each iteration. Thus we only need to {\em estimate} whether a \psc~is more likely or less likely to affect the final measurement results.
Our empirical evaluations suggest that our heuristics are effective, and much better than random pruning.

\subsection{Single-qubit single-Pauli-string cases}
We first study a simple case in which we can have more rigorous results. Suppose the ansatz has only one \ps~on one qubit. The lengths of the \ps s in the ansatz and the Hamiltonian are always 1.
\begin{enumerate}
    \item When the operator in the \ps~from the ansatz is $I$, we have $\bra{\psi}exp(-i\theta I)P exp(i\theta I)\ket{\psi} = \bra{\psi}P\ket{\psi}$ for any state $\psi$ and observable $P$. 
    This means applying the \psc~of \ps~$I$ does not change the measurement result. Actually $exp(i\theta I)$ is doing nothing but adding an invisible global phase.
    \item When the single-qubit \ps~observable from the Hamiltonian is $I$, we will have $\bra{\psi}exp(-i\theta P)I exp(i\theta P)\ket{\psi} = \bra{\psi}\ket{\psi} = 1$ for any $\psi$ and single-qubit \ps~$P$.
    This means when the measurement observable is $I$, applying \psc~of any operator does not change the measurement result, which is always $1$.
    \item When the operator in the Hamiltonian \ps~of the observable is the same with that in the ansatz \ps, we have  $\bra{\psi}exp(-i\theta P)P exp(i\theta P)\ket{\psi} = \bra{\psi}P\ket{\psi}$ for any $P\in\{X, Y, Z\}$.
    We have a geometrical explanation here.
    The state vector of a single qubit can be considered as a unit vector on the Bloch sphere in a three-dimensional  Euclidean vector space.
    $X, Y, Z$ can be considered as three orthogonal axes.
    When applying $exp(-i\theta P)$ ($P\in\{X, Y, Z\}$) on a state vector $\ket{\psi}$, the state vector on the Bloch sphere will rotate around the corresponding axis.
    Such rotation will not change the result when we project the state $\ket{\psi}$ onto the same axis.
    Therefore, the measurement result is not changed.
    \item When two operators from the \ps~of the Hamiltonian and the one in the ansatz are not the same (and they are not `I'), we have $\bra{\psi}exp(-i\theta P_a)P_H exp(i\theta P_a)\ket{\psi} \neq \bra{\psi}P_H\ket{\psi}$ for most $\ket{\psi}$ and $\theta$. 
    In this case, changing the parameter is very likely to affect the measurement result.
\end{enumerate}

\subsection{Multi-qubit multi-Pauli-string cases}

Now let us extend the discussion above to multi-qubit cases and multi-Pauli-string ansatz.
It is not easy to have precise results because one \psc~may be in the middle of the entire circuit and its rotation will also be affected by the follow-up gates.
Therefore, we only explain our high-level intuition here.
\begin{enumerate}
    \item When there are more `I's in the \ps~from the ansatz, this term is more unlikely to affect the state vector since fewer qubits are involved in the corresponding \psc.
    Therefore, we think such \psc s are less likely to affect final measurement result.
    \item When there are more `I's in the \ps~from the Hamiltonian, this measurement result of this term is less likely to be affected because the measurement results on those qubits with observable `I' will not affect the final results.
    \item When the two \ps s from the ansatz and the Hamiltonian share identical Pauli operators on more qubits, the effect of the rotation in the high-dimensional space is also reduced~(inspired by the case 3 in the last section).
\end{enumerate}

The Pauli string comparison rule in Section~\ref{sec:stringmatching} is designed based on this high-level intuition.
The experimental results in Section~\ref{sec:accuracyandconvergence} and Figure~\ref{fig:accuracy} empirically verified the effectiveness of this parameter importance estimation method.

\section{Experiment Configuration}\label{appendix:experiment}

The Hamiltonian of the simulated molecule is generated by PySCF~\cite{PYSCF} with STO-3G orbitals~\cite{hehre1969self} and Jordan-Wigner encoding~\cite{jordan1928paulische}.
We freeze the core electrons and only simulate the interaction of the outermost electrons.
We use the default UCCSD ansatz and the Variational Quantum Eigensolver~(VQE) from Qiskit Aqua library~(version 0.8.0).
The parameters are optimized using the Sequential Least Squares Programming (SLSQP)~\cite{kraft1988software} solver in SciPy~\cite{2020SciPy-NMeth}.
All the circuit simulations are performed with Qiskit Aer statevector simulator (version 0.6.0).
%The default compiler is Qiskit Terra~(version 0.15.0) with optimization level 3~(the highest level).
For the hardware yield rate, we adopt the yield simulation method and qubit frequency allocation algorithm in~\cite{li2020towards}.
All experiments are performed on a MacBook Pro with 2.8 GHz Quad-Core Intel Core i7 CPU and 16GB 2133MHz LPDDR3 memory.
